# Supplementary material for: IMDPrompter: Adapting SAM to Image Manipulation Detection by Cross-View Automated Prompt Learning
Source: arXiv:2502.02454 source file (2025-04-30)
Supplement: Supplementary file 1 [file X_suppl.tex]

\clearpage
\setcounter{page}{1}
\maketitlesupplementary

\section{Rationale}
\label{sec:rationale}
Having the supplementary compiled together with the main paper means that:
\begin{itemize}
\item The supplementary can back-reference sections of the main paper, for example, we can refer to \cref{sec:intro};
\item The main paper can forward reference sub-sections within the supplementary explicitly (e.g. referring to a particular experiment); 
\item When submitted to arXiv, the supplementary will already included at the end of the paper.
\end{itemize}
To split the supplementary pages from the main paper, you can use \href{https://support.apple.com/en-ca/guide/preview/prvw11793/mac#:~:text=Delete%20a%20page%20from%20a,or%20choose%20Edit%20%3E%20Delete).}{Preview (on macOS)}, \href{https://www.adobe.com/acrobat/how-to/delete-pages-from-pdf.html#:~:text=Choose%20%E2%80%9CTools%E2%80%9D%20%3E%20%E2%80%9COrganize,or%20pages%20from%20the%20file.}{Adobe Acrobat} (on all OSs), as well as \href{https://superuser.com/questions/517986/is-it-possible-to-delete-some-pages-of-a-pdf-document}{command line tools}.

\section{Experiment Details}
For hyper-parameters, we set $T_{nms,0}$=0.4, $T_0$=0.2, $T_0$=0.5, $T_1$=0.1, $\alpha$=0.9, $\beta$=0.9 on Activity v1.2 and v1.3. The T\_score was fine-tuned to 0.1 on THUMOS14, and the rest was consistent with the ActivityNet v1.2 and v1.3. All experiments were conducted on a single NVIDIA V100 GPU.
